# Supplementary material for: A Multimer Embedding Approach for Molecular Crystals up to Harmonic Vibrational Properties
Source: arXiv:2209.02687 ancillary file (2023-09-28)
Supplement: Supplementary file 1 [file supporting_information.pdf]

# Supporting Information for:

# A Multimer Embedding Approach for Molecular Crystals up to Harmonic Vibrational Properties

Johannes Hoja*[a], Alexander List[a], and A. Daniel Boese*[a]

[a] Department of Chemistry, University of Graz, Heinrichstraße 28/IV, 8010 Graz, Austria

* Correspondence to: johannes.hoja@uni-graz.at, adrian_daniel.boese@uni-graz.at

## Contents

**1 Number of Dimers and Trimers** **2**

**2 Lattice Energies** **3**

**3 Unit-Cell Volumes** **6**

**4 Phonon Densities of States** **8**

# 1 Number of Dimers and Trimers

**Table S1:** Number of identified unique dimers and trimers for a given cutoff distance for the X23 set evaluated on top of PBE0+MBD/light optimized structures; $Z$ lists the number of molecules within the unit cell and $n$ is the number of atoms per molecule.

| | | | Dimers | | | | | | Trimers | | | |
|---|---|---|---|---|---|---|---|---|---|---|---|---|
| | $n$ | $Z$ | 3 Å | 4 Å | 5 Å | 6 Å | 7 Å | 8 Å | 3 Å | 4 Å | 5 Å | 6 Å |
| 1,4-Cyclohexanedione | 16 | 2 | 6 | 8 | 9 | 14 | 20 | 28 | 8 | 16 | 20 | 51 |
| Acetic acid | 8 | 4 | 10 | 16 | 22 | 34 | 52 | 70 | 8 | 32 | 64 | 154 |
| Adamantane | 26 | 2 | 4 | 4 | 13 | 15 | 18 | 18 | 4 | 4 | 12 | 24 |
| Ammonia | 4 | 4 | 2 | 3 | 5 | 8 | 13 | 16 | 7 | 11 | 21 | 72 |
| Anthracene | 24 | 2 | 6 | 7 | 8 | 15 | 18 | 20 | 8 | 12 | 14 | 59 |
| Benzene | 12 | 4 | 6 | 6 | 9 | 14 | 20 | 28 | 8 | 8 | 20 | 51 |
| Carbon dioxide | 3 | 4 | 0 | 2 | 3 | 5 | 8 | 14 | 0 | 8 | 10 | 27 |
| Cyanamide | 5 | 8 | 10 | 15 | 18 | 43 | 56 | 72 | 6 | 28 | 40 | 260 |
| Cytosine | 13 | 4 | 4 | 7 | 10 | 17 | 21 | 28 | 2 | 12 | 25 | 79 |
| Ethyl carbamate | 13 | 2 | 13 | 15 | 19 | 35 | 41 | 53 | 20 | 28 | 46 | 166 |
| Formamide | 6 | 4 | 9 | 14 | 23 | 37 | 59 | 75 | 6 | 24 | 64 | 184 |
| Hexamine | 22 | 2 | 6 | 6 | 6 | 10 | 19 | 19 | 1 | 1 | 1 | 33 |
| Imidazole | 9 | 4 | 10 | 15 | 18 | 33 | 46 | 58 | 6 | 28 | 38 | 142 |
| Naphthalene | 18 | 2 | 6 | 7 | 8 | 17 | 18 | 21 | 8 | 12 | 14 | 77 |
| Oxalic acid $\alpha$ | 8 | 4 | 6 | 8 | 12 | 17 | 26 | 34 | 8 | 16 | 36 | 76 |
| Oxalic acid $\beta$ | 8 | 2 | 5 | 7 | 10 | 18 | 26 | 32 | 4 | 12 | 24 | 87 |
| Pyrazine | 10 | 2 | 4 | 5 | 5 | 11 | 13 | 20 | 4 | 7 | 7 | 39 |
| Pyrazole | 9 | 8 | 22 | 26 | 40 | 72 | 94 | 122 | 24 | 40 | 100 | 350 |
| *s*-Triazine[a] | 9 | 6 | 36 | 42 | 60 | 96 | 120 | 174 | 36 | 72 | 144 | 372 |
| *s*-Trioxane | 12 | 6 | 6 | 6 | 8 | 14 | 16 | 22 | 8 | 8 | 16 | 68 |
| Succinic acid | 14 | 2 | 5 | 7 | 11 | 16 | 24 | 31 | 4 | 12 | 28 | 68 |
| Uracil | 12 | 4 | 8 | 16 | 17 | 30 | 40 | 58 | 4 | 32 | 36 | 116 |
| Urea | 8 | 2 | 3 | 6 | 6 | 11 | 16 | 19 | 2 | 9 | 9 | 46 |

[a] Optimized without symmetry constraints.

## 2 Lattice Energies

**Table S2:** Lattice energies in kJ/mol calculated for the respective method with light species default settings on top of PBE0+MBD/light-optimized structures.

| System | PBE0+MBD | PBE+MBD | ME1 | ME2(3Å) | ME2(4Å) | ME2(5Å) | ME2(6Å) |
|---|---|---|---|---|---|---|---|
| 1,4-Cyclohexanedione | -99.6 | -92.7 | -95.0 | -96.5 | -95.6 | -95.6 | -95.7 |
| Acetic acid | -80.1 | -77.3 | -78.0 | -77.6 | -77.4 | -77.5 | -77.6 |
| Adamantane | -81.3 | -76.7 | -79.6 | -77.6 | -77.6 | -77.4 | -77.4 |
| Ammonia | -42.7 | -45.3 | -45.2 | -39.7 | -39.2 | -39.2 | -38.8 |
| Anthracene | -124.5 | -111.1 | -114.8 | -121.5 | -121.4 | -121.4 | -121.6 |
| Benzene | -60.4 | -56.2 | -57.4 | -57.8 | -57.8 | -57.8 | -57.8 |
| Carbon dioxide | -28.0 | -24.6 | -27.7 | -27.7 | -26.3 | -26.3 | -26.3 |
| Cyanamide | -90.5 | -92.1 | -92.9 | -87.8 | -87.0 | -86.9 | -86.7 |
| Cytosine | -171.5 | -164.5 | -164.6 | -165.7 | -167.3 | -167.8 | -168.0 |
| Ethyl carbamate | -95.1 | -91.1 | -93.4 | -92.0 | -91.7 | -91.3 | -91.2 |
| Formamide | -85.9 | -84.8 | -83.6 | -83.8 | -83.0 | -82.3 | -81.9 |
| Hexamine | -95.9 | -89.1 | -91.0 | -94.0 | -94.0 | -94.0 | -93.8 |
| Imidazole | -98.3 | -96.1 | -96.5 | -95.7 | -95.9 | -95.8 | -95.4 |
| Naphthalene | -91.6 | -82.8 | -85.2 | -88.7 | -88.5 | -88.5 | -88.7 |
| Oxalic acid $\alpha$ | -107.4 | -98.1 | -102.7 | -103.9 | -104.0 | -103.9 | -103.9 |
| Oxalic acid $\beta$ | -107.6 | -100.3 | -103.4 | -102.8 | -102.5 | -102.5 | -102.5 |
| Pyrazine | -69.5 | -65.8 | -67.4 | -65.1 | -66.5 | -66.5 | -66.4 |
| Pyrazole | -87.5 | -85.0 | -85.6 | -85.1 | -84.9 | -84.9 | -84.8 |
| $s$-Triazine | -64.0 | -58.7 | -60.7 | -59.0 | -60.4 | -60.2 | -60.3 |
| $s$-Trioxane | -70.6 | -63.7 | -65.8 | -66.1 | -66.1 | -66.1 | -66.0 |
| Succinic acid | -142.2 | -136.5 | -137.2 | -138.0 | -136.5 | -136.6 | -136.6 |
| Uracil | -147.2 | -139.8 | -140.3 | -142.3 | -143.3 | -143.3 | -143.5 |
| Urea | -112.5 | -109.8 | -110.1 | -110.6 | -109.0 | -109.0 | -107.8 |

**Table S3:** Lattice energies in kJ/mol calculated for the respective method with light species default settings on top of PBE0+MBD/light-optimized structures.

| System | ME2(7Å) | ME2(8Å) | ME3(3Å) | ME3(4Å) | ME3(5Å) | ME3(6Å) |
|---|---|---|---|---|---|---|
| 1,4-Cyclohexanedione | -95.7 | -95.7 | -99.6 | -100.0 | -100.0 | -100.2 |
| Acetic acid | -77.6 | -77.5 | -78.5 | -80.6 | -81.1 | -81.1 |
| Adamantane | -77.4 | -77.4 | -81.5 | -81.5 | -81.8 | -81.8 |
| Ammonia | -38.9 | -38.9 | -42.8 | -42.9 | -43.1 | -43.9 |
| Anthracene | -121.6 | -121.6 | -124.2 | -124.3 | -124.4 | -125.0 |
| Benzene | -57.8 | -57.8 | -60.2 | -60.2 | -60.7 | -61.0 |
| Carbon dioxide | -26.3 | -26.2 | -27.7 | -28.2 | -28.6 | -28.5 |
| Cyanamide | -86.7 | -86.6 | -90.0 | -91.5 | -91.9 | -91.5 |
| Cytosine | -167.5 | -166.8 | -167.2 | -171.7 | -172.4 | -173.5 |
| Ethyl carbamate | -91.2 | -91.3 | -95.3 | -95.6 | -95.7 | -95.9 |
| Formamide | -81.9 | -82.0 | -85.3 | -87.0 | -87.4 | -87.6 |
| Hexamine | -93.8 | -93.8 | -96.0 | -96.0 | -96.0 | -96.2 |
| Imidazole | -95.4 | -95.4 | -96.8 | -99.0 | -99.0 | -99.1 |
| Naphthalene | -88.6 | -88.6 | -91.4 | -91.5 | -91.6 | -92.2 |
| Oxalic acid $\alpha$ | -103.9 | -103.9 | -107.3 | -107.2 | -107.9 | -108.0 |
| Oxalic acid $\beta$ | -102.5 | -102.5 | -105.8 | -107.5 | -108.6 | -109.1 |
| Pyrazine | -66.3 | -66.4 | -66.7 | -69.9 | -69.9 | -70.3 |
| Pyrazole | -84.9 | -84.9 | -87.0 | -87.4 | -87.8 | -87.9 |
| *s*-Triazine | -60.3 | -60.2 | -61.1 | -64.5 | -64.7 | -64.7 |
| *s*-Trioxane | -66.3 | -65.9 | -69.4 | -69.4 | -70.0 | -70.0 |
| Succinic acid | -136.8 | -136.7 | -140.6 | -142.9 | -143.6 | -143.5 |
| Uracil | -143.4 | -143.5 | -143.9 | -147.8 | -147.8 | -148.2 |
| Urea | -108.9 | -109.1 | -113.0 | -113.1 | -113.1 | -112.4 |

**Table S4:** Lattice energies in kJ/mol calculated for the respective method with tight settings on top of PBE0+MBD/light-optimized structures.

| System | PBE0+MBD | PBE+MBD | ME1 | ME2(3Å) | ME2(4Å) | ME3(3Å) | ME3(4Å) |
|---|---|---|---|---|---|---|---|
| 1,4-Cyclohexanedione | -93.4 | -89.6 | -91.3 | -90.2 | -89.2 | -93.5 | -93.8 |
| Acetic acid | -76.4 | -74.8 | -74.9 | -74.4 | -73.8 | -75.5 | -77.0 |
| Adamantane | -79.3 | -77.7 | -80.6 | -75.2 | -75.2 | -79.4 | -79.4 |
| Ammonia | -40.8 | -42.5 | -42.3 | -37.9 | -37.3 | -41.2 | -41.8 |
| Anthracene | -110.8 | -103.8 | -107.0 | -107.1 | -106.9 | -110.9 | -111.1 |
| Benzene | -55.4 | -53.3 | -54.4 | -52.4 | -52.4 | -55.4 | -55.4 |
| Carbon dioxide | -24.5 | -21.8 | -23.6 | -23.6 | -22.7 | -23.6 | -24.6 |
| Cyanamide | -89.6 | -91.3 | -91.2 | -87.5 | -86.4 | -89.1 | -90.5 |
| Cytosine | -162.4 | -158.5 | -157.7 | -159.5 | -158.5 | -160.6 | -163.0 |
| Ethyl carbamate | -90.8 | -88.9 | -90.3 | -88.0 | -87.7 | -91.3 | -91.5 |
| Formamide | -82.2 | -81.4 | -79.5 | -81.2 | -79.8 | -82.3 | -83.7 |
| Hexamine | -89.5 | -85.9 | -88.3 | -85.1 | -85.1 | -89.8 | -89.8 |
| Imidazole | -92.3 | -91.8 | -91.7 | -90.4 | -89.9 | -91.4 | -93.1 |
| Naphthalene | -82.7 | -77.9 | -80.1 | -79.2 | -79.0 | -82.7 | -82.9 |
| Oxalic acid $\alpha$ | -98.5 | -91.7 | -94.1 | -95.5 | -95.5 | -98.5 | -98.3 |
| Oxalic acid $\beta$ | -98.7 | -93.8 | -94.9 | -95.3 | -94.5 | -97.6 | -98.9 |
| Pyrazine | -61.9 | -60.5 | -61.6 | -58.4 | -58.4 | -60.3 | -62.6 |
| Pyrazole | -81.5 | -80.7 | -80.6 | -79.2 | -78.9 | -81.3 | -81.6 |
| *s*-Triazine | -57.5 | -55.0 | -56.3 | -54.0 | -54.1 | -56.1 | -58.4 |
| *s*-Trioxane | -63.1 | -59.8 | -61.0 | -58.4 | -58.4 | -62.3 | -62.3 |
| Succinic acid | -135.5 | -131.5 | -131.4 | -131.7 | -130.2 | -134.3 | -136.0 |
| Uracil | -138.9 | -134.4 | -134.1 | -136.8 | -135.5 | -137.8 | -139.6 |
| Urea | -110.8 | -108.2 | -107.8 | -109.9 | -108.2 | -111.7 | -111.9 |

**Table S5:** Errors of the calculated lattice energies of the X23 set compared to PBE0+MBD. All energies were calculated using tight settings on top of the PBE0+MBD/light-optimized structures. The mean error (ME), the mean absolute error (MAE), and the maximal error (MAX) are given in kJ/mol while the mean relative error (MRE), the mean absolute relative error (MARE), and the maximal relative error (RMAX) are given in %.

| Method | ME | MAE | MAX | MRE | MARE | RMAX |
|---|---|---|---|---|---|---|
| PBE+MBD | 2.7 | 3.0 | 7.0 | -3.1 | 3.7 | 11.0 |
| ME1 | 1.8 | 2.2 | 4.8 | -1.8 | 2.4 | 4.5 |
| ME2(3Å) | 2.8 | 2.8 | 4.7 | -3.6 | 3.6 | 7.4 |
| ME2(4Å) | 3.4 | 3.4 | 5.3 | -4.4 | 4.4 | 8.6 |
| ME3(3Å) | 0.4 | 0.7 | 1.8 | -0.6 | 0.9 | 3.5 |
| ME3(4Å) | -0.5 | 0.5 | 1.4 | 0.6 | 0.7 | 2.4 |

# 3 Unit-Cell Volumes

**Table S6:** Unit-cell volumes in Å$^3$ calculated for the respective method with light species default settings.

| System | PBE0+MBD | PBE+MBD | ME1 | ME2(3Å) | ME2(4Å) | ME2(5Å) |
|---|---|---|---|---|---|---|
| 1,4-Cyclohexanedione | 271.3 | 280.7 | 278.3 | 274.7 | 275.8 | 275.8 |
| Acetic acid | 291.5 | 300.0 | 299.5 | 295.4 | 295.6 | 295.6 |
| Adamantane | 369.2 | 383.4 | 377.9 | 375.7 | 376.7 | 376.8 |
| Ammonia | 123.9 | 124.8 | 124.0 | 130.1 | 130.6 | 131.9 |
| Anthracene | 444.0 | 460.1 | 454.9 | 448.2 | 448.1 | 448.2 |
| Benzene | 453.2 | 469.0 | 464.1 | 461.0 | 461.0 | 461.0 |
| Carbon dioxide | 179.4 | 188.2 | 185.6 | 185.5 | 184.3 | 184.4 |
| Cyanamide | 411.4 | 422.4 | 417.1 | 422.8 | 430.2 | 428.8 |
| Cytosine | 457.6 | 478.8 | 474.3 | 475.5 | 466.1 | 465.6 |
| Ethyl carbamate | 237.2 | 245.1 | 242.2 | 240.5 | 240.4 | 240.9 |
| Formamide | 218.1 | 224.7 | 224.6 | 224.8 | 224.5 | 225.5 |
| Hexamine | 314.6 | 330.1 | 324.6 | 321.9 | 321.9 | 321.9 |
| Imidazole | 344.7 | 358.3 | 355.2 | 354.9 | 353.3 | 353.7 |
| Naphthalene | 333.7 | 346.1 | 342.1 | 337.8 | 337.8 | 337.9 |
| Oxalic acid $\alpha$ | 303.3 | 315.9 | 314.5 | 307.1 | 307.1 | 307.1 |
| Oxalic acid $\beta$ | 152.5 | 159.4 | 158.6 | 155.7 | 155.9 | 155.9 |
| Pyrazine | 191.9 | 201.0 | 199.2 | 200.2 | 198.7 | 198.7 |
| Pyrazole | 689.8 | 717.8 | 711.3 | 701.8 | 702.1 | 702.3 |
| *s*-Triazine | 549.1 | 567.2 | 563.4 | 562.8 | 558.7 | 559.6 |
| *s*-Trioxane | 575.2 | 611.5 | 606.7 | 600.3 | 600.3 | 600.4 |
| Succinic acid | 237.3 | 246.4 | 244.3 | 241.4 | 241.8 | 241.9 |
| Uracil | 445.8 | 462.7 | 459.1 | 455.2 | 450.7 | 451.0 |
| Urea | 140.5 | 144.1 | 143.7 | 142.8 | 143.4 | 143.4 |

**Table S7:** Unit-cell volumes in Å$^3$ calculated for the respective method with tight settings.

| System | PBE0+MBD | PBE+MBD | ME1 | ME2(3Å) | ME2(4Å) |
|---|---|---|---|---|---|
| Acetic acid | 292.4 | 298.5 | 298.0 | 296.3 | 296.9 |
| Ammonia | 124.1 | 125.2 | 125.0 | 128.5 | 129.1 |
| Carbon dioxide | 182.6 | 190.7 | 188.5 | 188.5 | 186.6 |
| Ethyl carbamate | 237.2 | 242.2 | 240.2 | 239.7 | 240.2 |
| Oxalic acid $\beta$ | 154.1 | 159.6 | 158.6 | 156.2 | 156.9 |
| Pyrazine | 197.6 | 201.6 | 200.0 | 201.2 | 200.6 |
| Succinic acid | 238.7 | 245.4 | 243.8 | 241.9 | 242.3 |
| Urea | 141.9 | 144.2 | 143.7 | 142.3 | 143.0 |

**Table S8:** Errors of calculated cell volumes (in % ) of a reduced set containing 8 systems from X23 calculated with tight settings compared to PBE0+MBD results.

| Method | MRE | MARE | RMAX |
|---|---|---|---|
| PBE+MBD | 2.5 | 2.5 | 4.4 |
| ME1 | 1.8 | 1.8 | 3.2 |
| ME2(3Å) | 1.8 | 1.8 | 3.5 |
| ME2(4Å) | 1.8 | 1.8 | 4.1 |

## 4 Phonon Densities of States

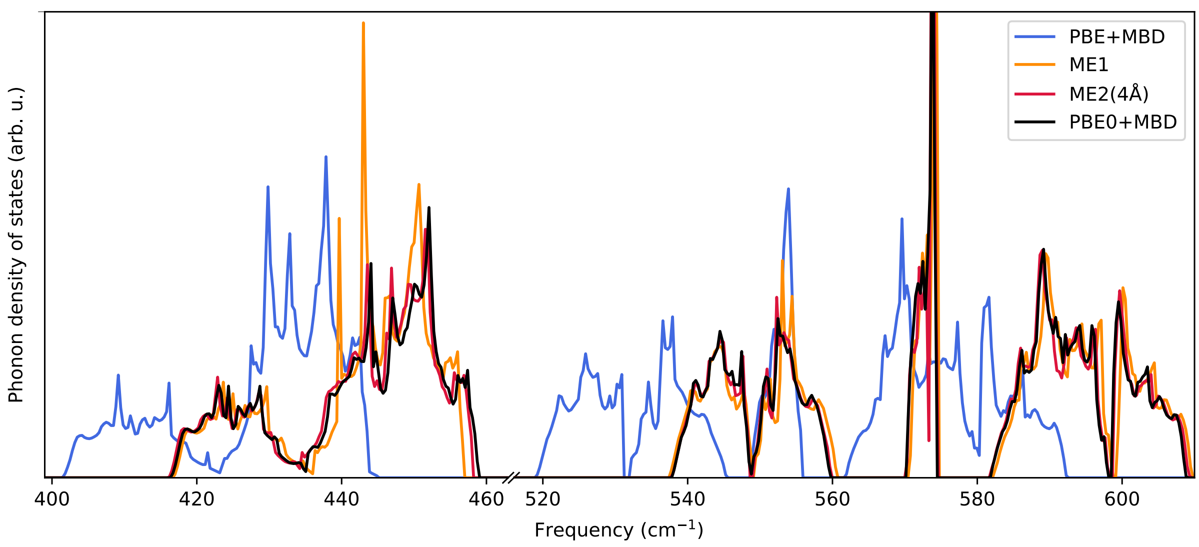


**Figure S1:** Phonon density of states of uracil calculated on top of internally relaxed structures using the PBE0+MBD/light lattice vectors for several methods (only frequencies between 400 and 610 cm$^{-1}$ are shown).

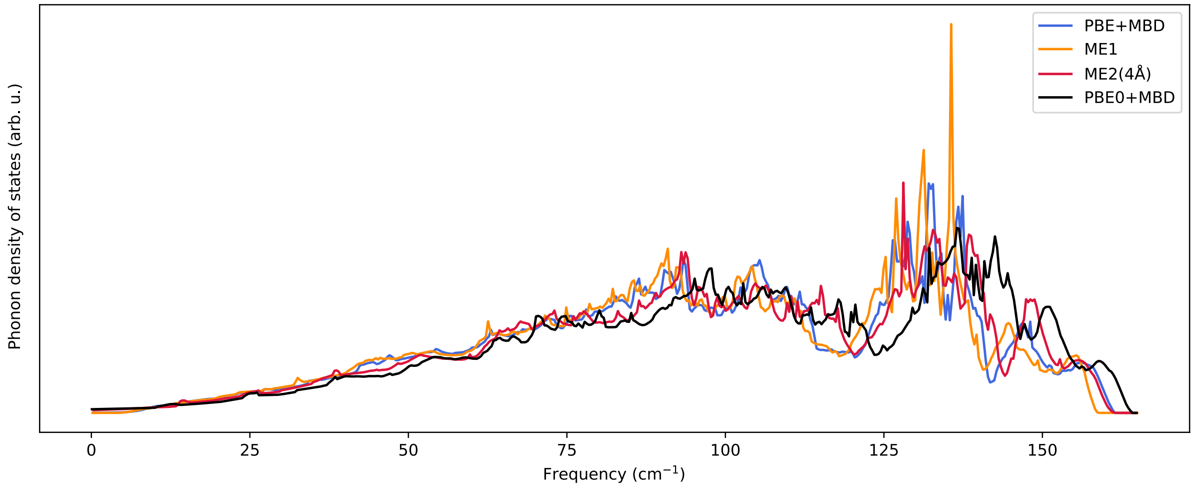


**Figure S2:** Low-frequency phonon density of states of uracil calculated on top of optimized structures for several methods.

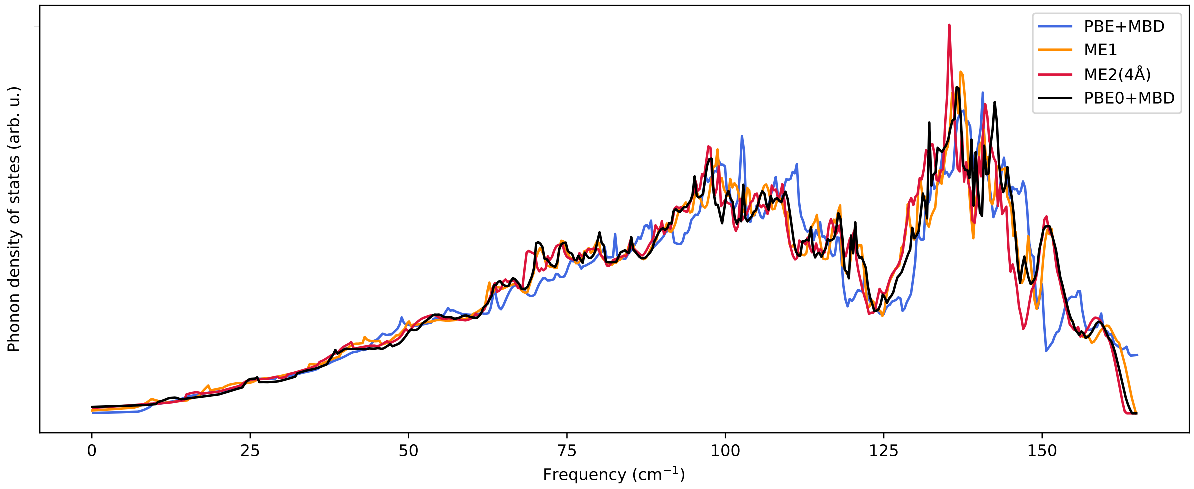


**Figure S3:** Low-frequency phonon density of states of uracil calculated on top of internally relaxed structures using the PBE0+MBD/light lattice vectors for several methods.
